# Supplementary material for: Duwak: Dual Watermarks in Large Language Models
Source: arXiv:2403.13000 source file (2024-08-08)
Supplement: Supplementary file 1 [file proof.tex]

\clearpage
% \newpage
% \section{Proofs}
% \begin{definition}[Spike Entropy]
% Given a discrete probability vector \(p\) and a scalar \(z\), the spike entropy of \(p\) with respect to \(z\) is defined as
% \[
% S(p, z) = \sum^n \frac{p^n}{1 + z p^n}.
% \]
% \end{definition}
